# Supplementary material for: Unsupervised BatchNorm Adaptation (UBNA): A Domain Adaptation Method for Semantic Segmentation Without Using Source Domain Representations
Source: arXiv:2011.08502 source file (2021-11-11)
Supplement: Supplementary file 1 [file method.tex]

\section{Additional Method Details}

In this section we describe the pre-training of our semantic segmentation model. Note, that we describe this only for completeness and that in principle any pre-training of the semantic segmentation is compatible with our \textbf{UBNA} method. 

\subsection{Semantic Segmentation}
\label{sec:semantic_segmentation}

The semantic segmentation relies on a single input image $\boldsymbol{x}\in\mathbb{I}^{H\times W\times C}$, where $H$ defines the height, $W$ the width, and $C=3$ the number of color channels. The range $\mathbb{I} = \left[0,1\right]$ defines the normalized range of gray values. At inference, the neural network is used to predict a pixel-wise semantic segmentation map $\boldsymbol{m} \in \mathcal{S}^{H\times W}$ from the single image $\boldsymbol{x}$. Here, $\mathcal{S}$ is the set of considered semantic classes.
\par
The semantic segmentation is trained by supervision from ground truth labels $\overline{\bm{m}}= \left(\overline{m}_{i}\right)\in\mathcal{S}^{H\times W}$, which are utilized in a one-hot encoded fashion as $\overline{\bm{y}} = \left(\overline{y}_{i,s}\right)\in \left\lbrace 0,1\right\rbrace^{H\times\ W\times |\mathcal{S}|}$, such that $\overline{m}_{i} = \argmax_{s \in \mathcal{S}} \overline{y}_{i, s}$ at each pixel index $i \in \mathcal{I} = \left\lbrace 1, ..., H\cdot W\right\rbrace$ in the image. During training, the network then predicts output probabilities $\boldsymbol{y} = \left(y_{i, s}\right) \in\mathbb{I}^{H\times W\times |\mathcal{S}|}$ with the number $|\mathcal{S}|$ of semantic classes, which are optimized utilizing the cross-entropy loss
\begin{equation}
J^{\mathrm{seg}}\left( \boldsymbol{y}, \overline{\bm{y}}\right) = -\frac{1}{H\cdot W}\sum_{i \in\mathcal{I}}\sum_{s \in\mathcal{S}} w_s \overline{y}_{i,s} \cdot \log\left(y_{i,s}\right), 
\label{eq:crossentropy_loss}
\end{equation}
where $w_s$ are the class weights as defined in \cite{Paszke2016}. The final pixel-wise classes are then obtained by $m_{i} = \argmax_{s \in \mathcal{S}} y_{i, s}$, yielding the estimated segmentation mask $\boldsymbol{m} = \left(m_{i}\right)\in \mathcal{S}^{H\times W}$.
